# Supplementary material for: Glass-like dynamics of the strain-induced coil/helix transition on a permanent polymer network
Source: arXiv:1601.07706 source file (2016-01-28)
Supplement: Supplementary file 1 [file Supplemental.pdf]

# Supplemental Material

## I. SCALING REGIMES OF THE SPECIFIC VISCOSITY

The viscosity of gelatin aqueous solutions was measured using a double gap Couette cell geometry at temperature $T = 40°$ C where gelatin is in the coil state. Figure 1 shows the specific viscosity $(\eta(c) - \eta_S)/\eta_S$ as a function of concentration $c$, where $\eta$ is the viscosity of the solution in the Newtonian regime (typically $\dot{\gamma} \leq 1$ s$^{-1}$) and $\eta_S$ is the solvent (water) viscosity.

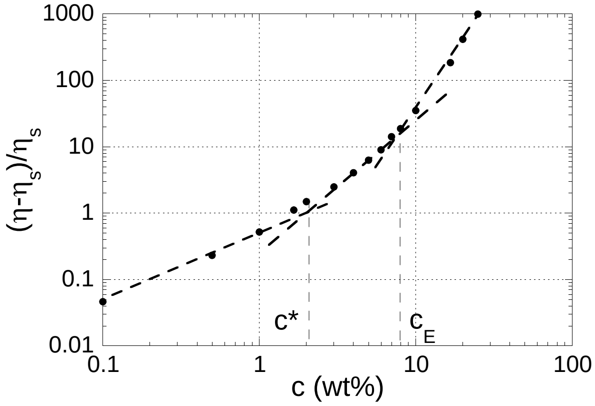


FIG. 1. Intrinsic viscosity of gelatin solutions *vs* concentration, measured at $T = 40°$ C. The boundaries between the three scaling regimes define the overlap $c^\star = 2$ wt.% and entanglement $c_E = 8$ wt.% concentrations.

The three usual scaling regimes of polymer solutions are observed :

- dilute regime where $\eta_{\rm sp} \sim c$ at low concentrations $c < c^\star$.
- semi-dilute non entangled regime at intermediate concentrations $c^\star < c < c_E$. There, $\eta_{\rm sp} \sim c^2$, as expected for a solution in $\theta$-solvent. Indeed, the Flory-Huggins interaction parameter $\chi$ for gelatin aqueous solutions is $0.49 \pm 0.01$, very close to 0.5, the $\theta$-solvent value[1].
- entangled regime where $\eta_{\rm sp} \sim c^{3.5}$ at high concentrations $c > c_E$.

The measured scaling exponents agree with those reported by Guo et al. [2]. However, the values of the overlap and entanglement concentrations $c^\star = 2$ wt.% and $c_E = 8$ wt.%, are significantly different from theirs. We assign this difference to the fact that these authors were using gelatin of type B whereas our work has been conducted on type A. These two polyelectrolytes obtained by different collagen denaturation routes have different content of ionizable residues, as witnessed by the difference between their isoelectric points ($pI_A = 9, pI_B = 5$ at 40° C). We therefore expect their rigidities to be different.

From the above results, we conclude that the $c = 5$ wt.% solutions used in the present work lie in the semi-dilute non-entangled regime. We can thus exclude relaxation mechanisms associated with entanglements in the polymer network.

## II. THERMAL REVERSIBILITY

If the stress relaxation which we observe does result from a strain induced coil-helix transition, this relaxation should be fully reversible upon heating the strained system above the transition temperature of the strands. In order to check this reversibility, we performed the following experiments on gels of target modulus $G = 1400$ Pa.

A first sample is sheared with a deformation $\epsilon = 50\%$ at temperature $T_1 = 55°$ C. No significant relaxation is observed, from which we conclude that $T_1$ lies above the coil-helix transition of the strained gel. The stress level is measured to be $\sigma_1 = 815$ Pa.

A second sample is then sheared up to the same strain level $\epsilon = 50\%$ at $T_2 = 35°$ C, where significant relaxation does occurs. After waiting for full relaxation, the temperature is suddenly increased to $T_1 = 55°$ C while maintaining the strain. As shown on figure 2, the stress increases and rapidly reaches a constant value $\sigma_2 = 818$ Pa.

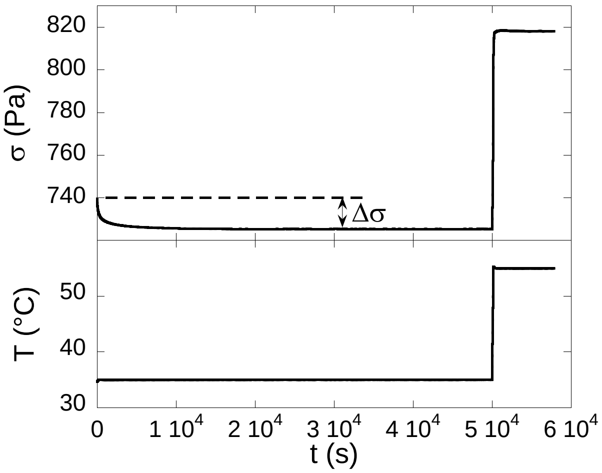


FIG. 2. Response of a $G = 1400$ Pa sample following (i) a strain step of magnitude $\epsilon = 50\%$ applied at $t = 0$, (ii) a temperature step applied after full relaxation at the initial temperature. Upper panel: stress response. Lower panel: Thermal history.

The difference between $\sigma_1$ and $\sigma_2$ is fully compatible with the scattering of the shear moduli values for different samples which we have determined (on a set of 6 samples) to be $\delta G = \pm 6$ Pa yielding $\delta\sigma = \epsilon\delta G = \pm 3$ Pa. So we can conclude, within experimental uncertainty, to the thermal reversibility of the relaxation process. By the same token, this result also proves that no significant wall slip occurs under the 50% strain applied here.

## III. NETWORK MODEL

We adapt the network model of ref [3] to the case of simple shear deformations, assuming that the quenched distribution of end-to-end distances $\mathbf{R}$ between cross-links obeys a gaussian distribution

$$P(\mathbf{R}) \propto \exp\left(-\frac{3\mathbf{R}^2}{2Na^2}\right)$$

where $a$ is the monomer size and $N$ the number of monomers.

A strand at azimuthal angle $\varphi$ and a polar angle $\vartheta$ having an initial end-to-end vector $\mathbf{R}$ will, under shear deformation $\epsilon$ in the $x$ direction, have a end-to-end vector $\mathbf{R}'$ (see Figure 3) and thus be stretched to a length $\eta R$ with

$$\eta = \sqrt{1 + \epsilon\cos\vartheta(\epsilon\cos\vartheta + 2\sin\vartheta\cos\varphi)}$$

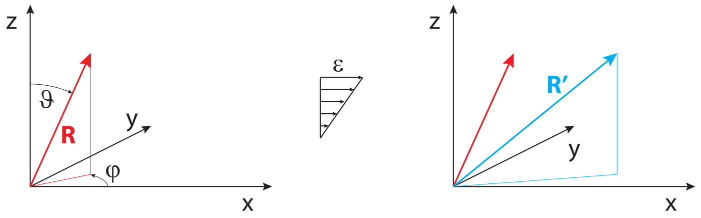


FIG. 3. Change in end-to-end vector consecutive to a shear strain $\epsilon$.

Using the dimensionless parameters introduced in Section IV.A of the main text and the notations of Figure 6, the tension $\phi_B(x,\eta)$ following the shear and the equilibrium tension $\phi_C(x,\eta)$ are given by:

$$\phi_B(x,\eta) = \begin{cases} \dfrac{3k_BT}{a}\eta x & x < x_- \text{ or } x > x_+ \\ \dfrac{3k_BT}{a}\left(x_- + x\dfrac{\eta - 1}{|\gamma - x|}(\gamma - x_-)\right) & x_- < x < x_+ \end{cases} \tag{1}$$

$$\phi_C(x,\eta) = \begin{cases} \frac{3k_BT}{a}\eta x & x < x_- \text{ or } x > x_+ \\ \frac{3k_BT}{a}x_- & x_- < \eta x < \gamma \\ \frac{3k_BT}{a}x_+ & \gamma < \eta x < x_+ \end{cases} \quad (2)$$

Integrating on strand directions and lengths, the total force along the shear direction $x$ reads:

$$\Phi_{B,C} = \iiint p(x)\phi_{B,C}(x,\eta)\frac{\sin\vartheta\cos\varphi + \epsilon\cos\vartheta}{\eta}x^2\sin\vartheta d\vartheta d\varphi dx$$

which can be computed numerically for both $\phi_B$ and $\phi_C$. The relative shear force drop $\Delta\Phi/\Phi_B = (\Phi_B - \Phi_C)/\Phi_B$ can thus be computed as a function of $\theta$ (eq. (2) of the main text), which increases linearly with temperature. Figure 4 shows the dependence of $\Delta\Phi/\Phi_B$ on $\theta$ obtained using the following parameter values: $\epsilon = 0.2$, $N = 100$, $\gamma = 0.4$.

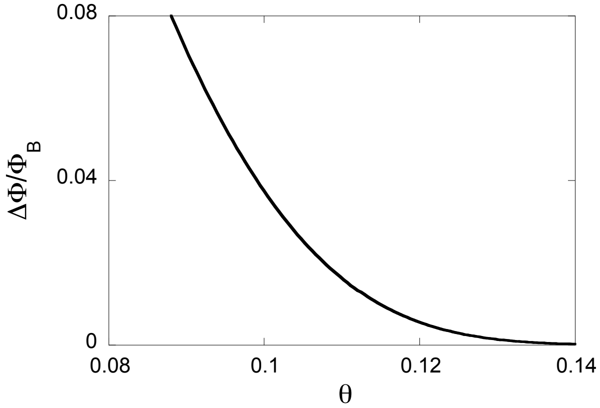


FIG. 4. Relative shear force drop versus reduced temperature $\theta$, computed for $\epsilon = 0.2$, $\gamma = 0.4$ and $N = 100$.

Assimilating $\Delta\Phi/\Phi_B$ to the relative stress drop $\Delta\sigma/\sigma_0$ and keeping in mind that $\theta$ is a linear function of $T$, though with an unknown coefficient $C$ (see main text), we recover the gradual nature of the transition to the fully coiled state which is a qualitative feature of our experimental results (Fig. 6). A more quantitative comparison is precluded by the crudeness of the model assumptions, in particular that of a gaussian end-to-end distribution and, probably more serious, of the mechanical independence of the strands.

[1] H. B. Bohidar and S. S. Jena, *J. Chem. Phys.* **100**, 6888 (1994).
[2] L. Guo, R. H. Colby, C. P. Lusignan, and A. M. Howe, *Macromol.* **36**, 10009 (2003).
[3] S. Kutter and E.M. Terentjev, *Eur. Phys. J. E* **8**, 539 (2002).
